# Supplementary material for: Repopulating Street Scenes
Source: arXiv:2103.16183 source file (2021-03-30)
Supplement: Supplementary file 1 [file 08-suppl.tex]

\newpage

\begin{table*}[t!]
    \centering
    \begin{tabular}{lcccc}
    \toprule
    Method & All & Sunny & Cloudy & SSIM \\
    \midrule
    Shadow-free composite & 0.0183 & 0.0140 & 0.0124 & 0.029\\
    Shadow network~\cite{wang2020people} & 0.0171 & 0.0125 & 0.0117 & 0.029 \\
    Ours (w/o depth map) & 0.0189 & 0.0133 & 0.0125 & 0.028\\
    Ours (w/o sun position) & \textbf{0.0164} & 0.0117 & \textbf{0.0109} & 0.029\\
    % Ours (w/o $x$-$y$ grid) & 0.0195 & 0.0141 & 0.0141  & 0.029\\
    Ours & \textbf{0.0165} & \textbf{0.0116} & \textbf{0.0109}  & 0.029\\
    % \toprule
    % Method & LPIPS & SSIM \\
    % \midrule
    % Shadow network & 0.0171 & 0.029 \\
    % Ours (w/o depth map) & 0.0189 & 0.028\\
    % Ours (w/o sun position) & \textbf{0.0164} & 0.029\\
    % Ours & \textbf{0.0165} & 0.029\\
    \bottomrule
    \end{tabular}
    \vspace{3pt}
    \caption{Object insertion results for cropped object regions, on all test images, as well as the sunny subset, and the cloudy subset, measured in LPIPS~\cite{zhang2018unreasonable} and SSIM. Lower is better.}
    \label{tbl:insert_bbox}
\end{table*}

\begin{table}[t!]
    \centering
    \begin{tabular}{lccc}
    \toprule
    Method  & All & Sunny & Cloudy \\
    \midrule
    Input                       & 0.085          & 0.087         & 0.084 \\
    CRA~\cite{yi2020contextual} & 0.076          & 0.077         & 0.075 \\
    Ours                        & \textbf{0.057} & \textbf{0.058} & \textbf{0.057} \\
    \bottomrule
    \end{tabular}
    \vspace{3pt}
    \caption{Object removal results for cropped object regions, on all test images, as well as the sunny subset, and the cloudy subset, measured in LPIPS~\cite{zhang2018unreasonable}. Lower is better.}
    \label{tbl:removal_bbox}
\end{table}

\begin{table}[t!]
    \centering
    \begin{tabular}{lc}
    \toprule
    Method  & All \\
    \midrule
    Input               & 0.085 \\
    CRA~\cite{yi2020contextual} (w/ our mask)   & 0.078 \\
    Ours (w/o mask)     & 0.074 \\
    Ours (w/o flow)     & 0.061 \\
    Ours                & \textbf{0.057} \\
    \bottomrule
    \end{tabular}
    \vspace{3pt}
    \caption{Object removal results for cropped object regions on all test images, measured in LPIPS~\cite{zhang2018unreasonable}. Lower is better.}
    \label{tbl:removal_bbox_abla}
\end{table}

\section{Implementation Details}
\subsection{Data}
We collected short (stationary camera) image bursts of street scenes from Google Street View, captured between 2014 and 2020. Using GPS and structure from motion, we identified image bursts coming from parked Street View cars. The cooldown between each capture is about five seconds. The training image bursts were captured in major US cities, including San Francisco, Seattle, Los Angeles, San Jose, New York City, Boston, Chicago and Phoenix. 
We also collected a test set from nearby cities, including Jersey City, Brooklyn, Berkeley, San Diego, Long Beach and Pittsburgh, to ensure there is no overlap with the training set. 
Each image burst consists of at least 10 images. 
Given an image stack, we calculated the median image by taking the channel-wise median value per pixel for the whole stack.
We used the median image of the bursts as a ``clean plate,'' free of moving objects and their shadows (we also refer to this image as the ``background image''). In total, we collected 142,778 image/background pairs for training and 16,034 as a test set. 

We use Mask R-CNN~\cite{wu2019detectron2} as our instance segmentation network, and set its confidence threshold Mask R-CNN to 0.6 to keep the partially occluded objects. For class maps used in the removal and insertion network, we segment out the following classes that often represent moving objects (or parts of moving objects) in street scenes: 
person, bicycle, car, motorcycle, airplane, train, bus, truck, boat, bird, cat, dog, backpack, handbag, tie, suitcase, and skateboard. 
We compare the objects detected in the input image and in the background image to determine whether an object is moving. If a bounding box in the input image has an IOU (intersection-over-union) of more than $0.6$ with a bounding box in the background image, we consider this object to be static (not moving), and thus do not include it in the class mask.
Finally, we only use an image for training if its class mask's area is more than $1\%$ of the whole frame.

\subsection{Removal Network}
The generator component of our removal network is inspired by~\cite{johnson2016perceptual}. It has three branches of residual blocks predicting the inpainting mask, appearance flow, and high-dimensional features respectively. Each branch has $5$ residual blocks. 
The supervision for the inpainting mask is computed by thresholding the color difference between the median image and the original image. We assume such differences are caused by moving objects and their shadows.
We use the ``clean plate'' median background image as the ground truth image to be predicted. 
The loss function consists of two multi-scale discriminators with LSGAN loss, a feature matching loss, a VGG perceptual loss for the object/shadow removed image, and a cross-entropy loss for the inpainting mask.
The initial learning rate is set to 1e-5 for 25 epochs and then decays linearly to 0 over another 25 epochs. We use the Adam optimizer and a batch size of 8. We train our network on eight NVIDIA Tesla P100 GPUs; it takes three days to train.

\subsection{Sun Estimation Network}
Based on the time and location of an image, we calculate the ground truth sun position using solar equations. We then convert this sun position to two one-hot vectors as the ground truth supervision for sun azimuth and elevation angle. The sun estimation network uses a similar structure as a ResNet50 network~\cite{he2016deep}, where the last fully connected layer is replaced with two, one for azimuth and one for elevation. This network is trained with a cross-entropy loss with a smooth coefficient of $0.1$. We use the SGD optimizer with a learning rate of 1e-3. We train the network for 20 epochs with batch size 64. We train on eight NVIDIA Tesla P100 GPUs for one day.

\subsection{Insertion Network}
The generator component of the insertion network is also inspired by~\cite{johnson2016perceptual}. It has five residual blocks, followed by two transposed convolution upsampling branches, one for the bias map and one for the gain map. We use the original street image as ground truth supervision. The loss function is the same as in~\cite{wang2018high}, i.e., two multi-scale discriminators with LSGAN loss, a feature matching loss, and a VGG perceptual loss. The initial learning rate is set to 1e-4 for 15 epochs and then decays linearly to 0 over another 15 epochs. We use the Adam optimizer and a batch size of 8. We train our network on eight NVIDIA Tesla P100 GPUs, and it takes three days to train.

\subsection{Timing for Each Network}
At test time, the sun estimation network takes $50$ms per image on an NVIDIA Titan Xp, and the removal and insertion networks take $150$ms.

\section{Additional Experiments}
\subsection{Removal Network}
\label{sec:removal_addi}
We found that shadows only occupy a small portion of the whole frame. Therefore, as an additional evaluation protocol, we center crop out the object region using a square that is 1.5 times the bounding box size to further evaluate the performance of the removal network, focused on the object and its surroundings (including its shadow), as opposed to unmodified parts of the image far from objects. We evaluated on all the test images as well as the sunny and cloudy subset ($\sim$150 images each).
Quantitative results on cropped regions are shown in Table~\ref{tbl:removal_bbox}. Our method has a clear advantage over the traditional inpainting method~\cite{yi2020contextual}. Unlike in standard inpainting, our model automatically detect and remove hard and soft shadows, not just masked objects.

Additional ablations on our removal network are shown in Table~\ref{tbl:removal_bbox_abla}. We compared our full removal network with 1) CRA~\cite{yi2020contextual} using our (thresholded) inpainting mask; 2) ours without inpainting mask; and 3) ours without flow map.
These results demonstrate the effectiveness of the inpainting mask and flow map modules.
Note that our inpainting mask is trained end-to-end with our flow-map inpainter, which offers advantages over separately trained modules: though there may be errors in mask estimation, the inpainter is trained to handle them when recombined to create the final object/shadow-removed image.  An interesting area of future work is to incorporate and train different inpainting algorithms (in addition to our flow map method) end-to-end within our network.

Additional qualitative results are shown in Figure~\ref{fig:remove_suppl}.

% We show additional qualitative results for the task of removing objects in Figure~\ref{fig:remove_suppl}. These results demonstrate how, unlike in standard inpainting, our method can automatically detect and remove shadows, not just masked objects.

\subsection{Insertion Network}
The insertion network only modifies a small part of the fully image.  However, common metrics like FID, SSIM, and LPIPS, compare image-level statistics.
Accordingly, in Table~\ref{tbl:insert_bbox} we report LPIPS and SSIM scores on crops around inserted objects, as described in Section~\ref{sec:removal_addi}.  The gains over ``shadow network''~\cite{wang2020people} are clearer with cropped LPIPS; w/ and w/o sun position still have similar LPIPS scores; and SSIM suggests minimal differences. Ultimately, we think these numbers illustrate challenges with the metrics themselves. In practice, we find the depth map and sun position appreciably improve overall visual quality, leading to fewer detached or broken shadows in Figure~\ref{fig:insert_suppl}, something these metrics are evidently not attuned to.

We show additional qualitative results for the task of inserting objects in Figure~\ref{fig:insert_suppl}. Our method has an advantage over other models. On sunny days, our full model benefits from the depth map, sun position and $x$-$y$ grid and outputs realistic shadows with details. On cloudy days, our model synthesize subtle soft shadows, still performing the best among all methods and ablations.

\subsection{Repopulating Street Scenes}
We show additional qualiitative results for the full task of repopulating street scenes (involving removal, sun position estimation, and insertion) in Figure~\ref{fig:repop_suppl}.

\begin{figure*}[t]
    \centering
    \includegraphics[width=.75\linewidth]{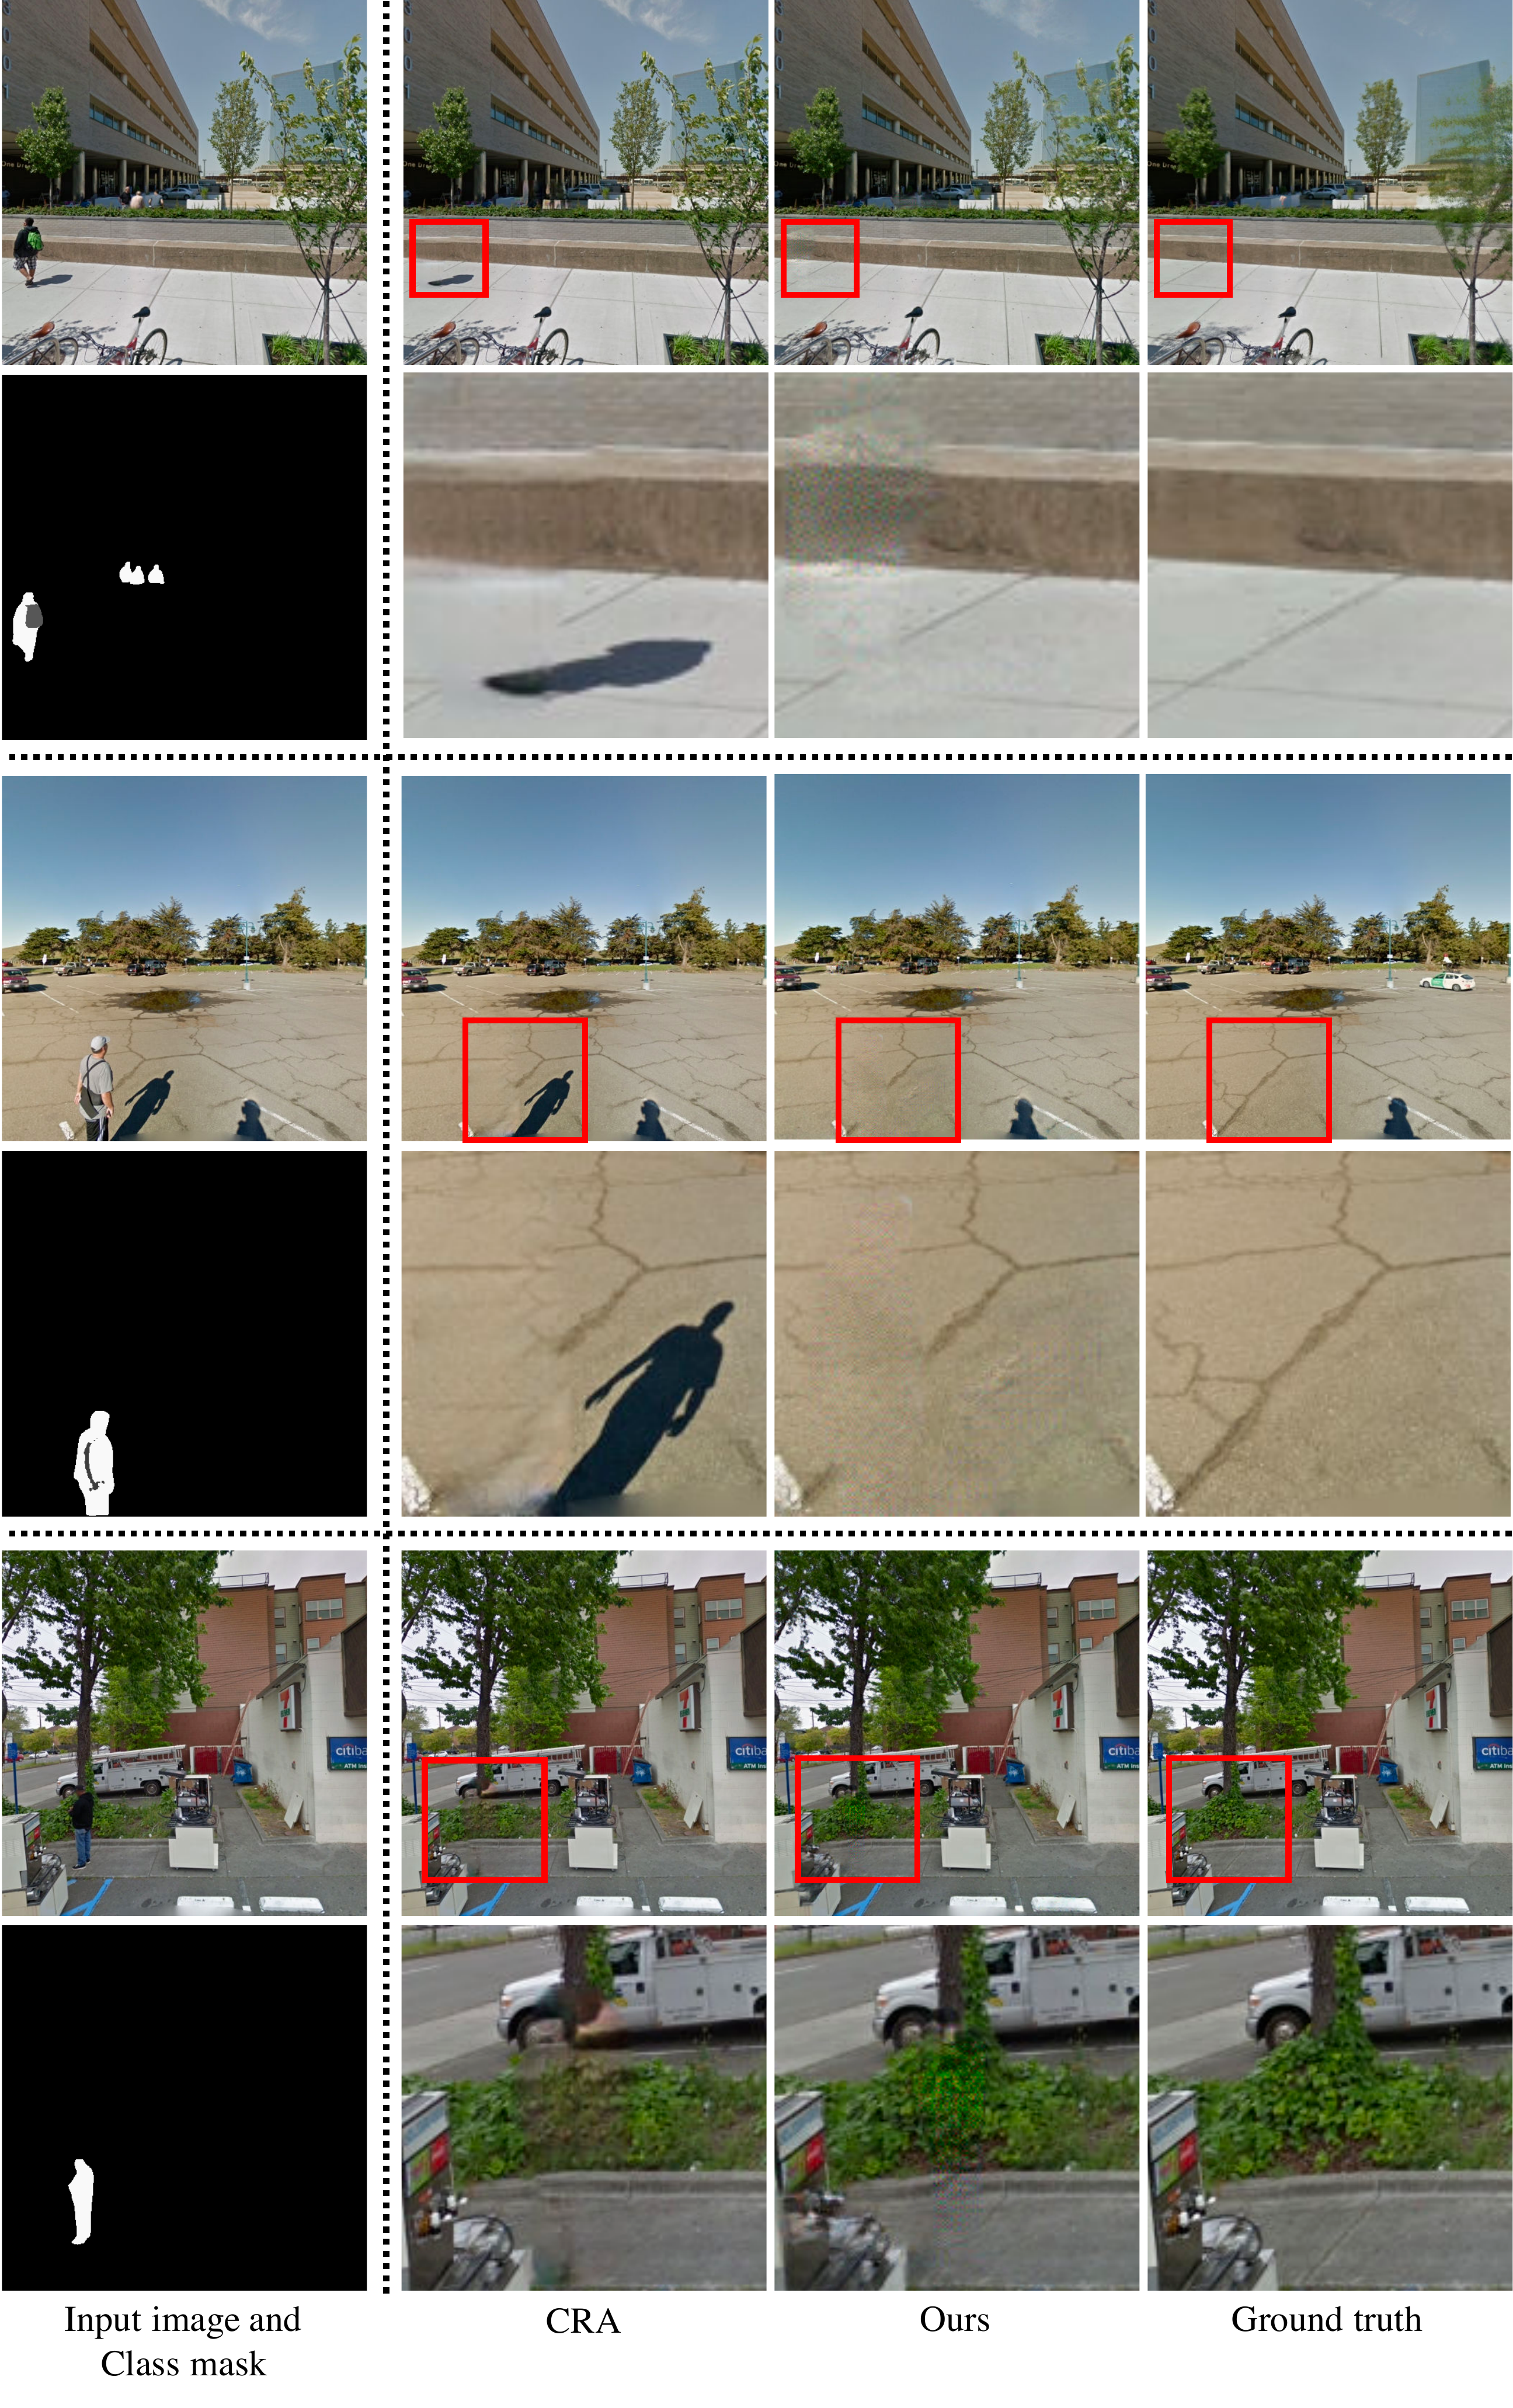}
    \caption{Object removal results on the test set.  Three examples are shown, with red boxes indicating close-up regions (inset regions are shown in a row below the full images). The traditional inpainting method~\cite{yi2020contextual} only inpaints the area within the mask and leaves leftover shadows. Our method removes objects completely along with their shadows. In addition, the prior inpainting method can fail in the case of large objects (such as the tree in the last example).}
    \label{fig:remove_suppl}
\end{figure*}

\begin{figure*}[t]
    \centering
    \includegraphics[width=\linewidth]{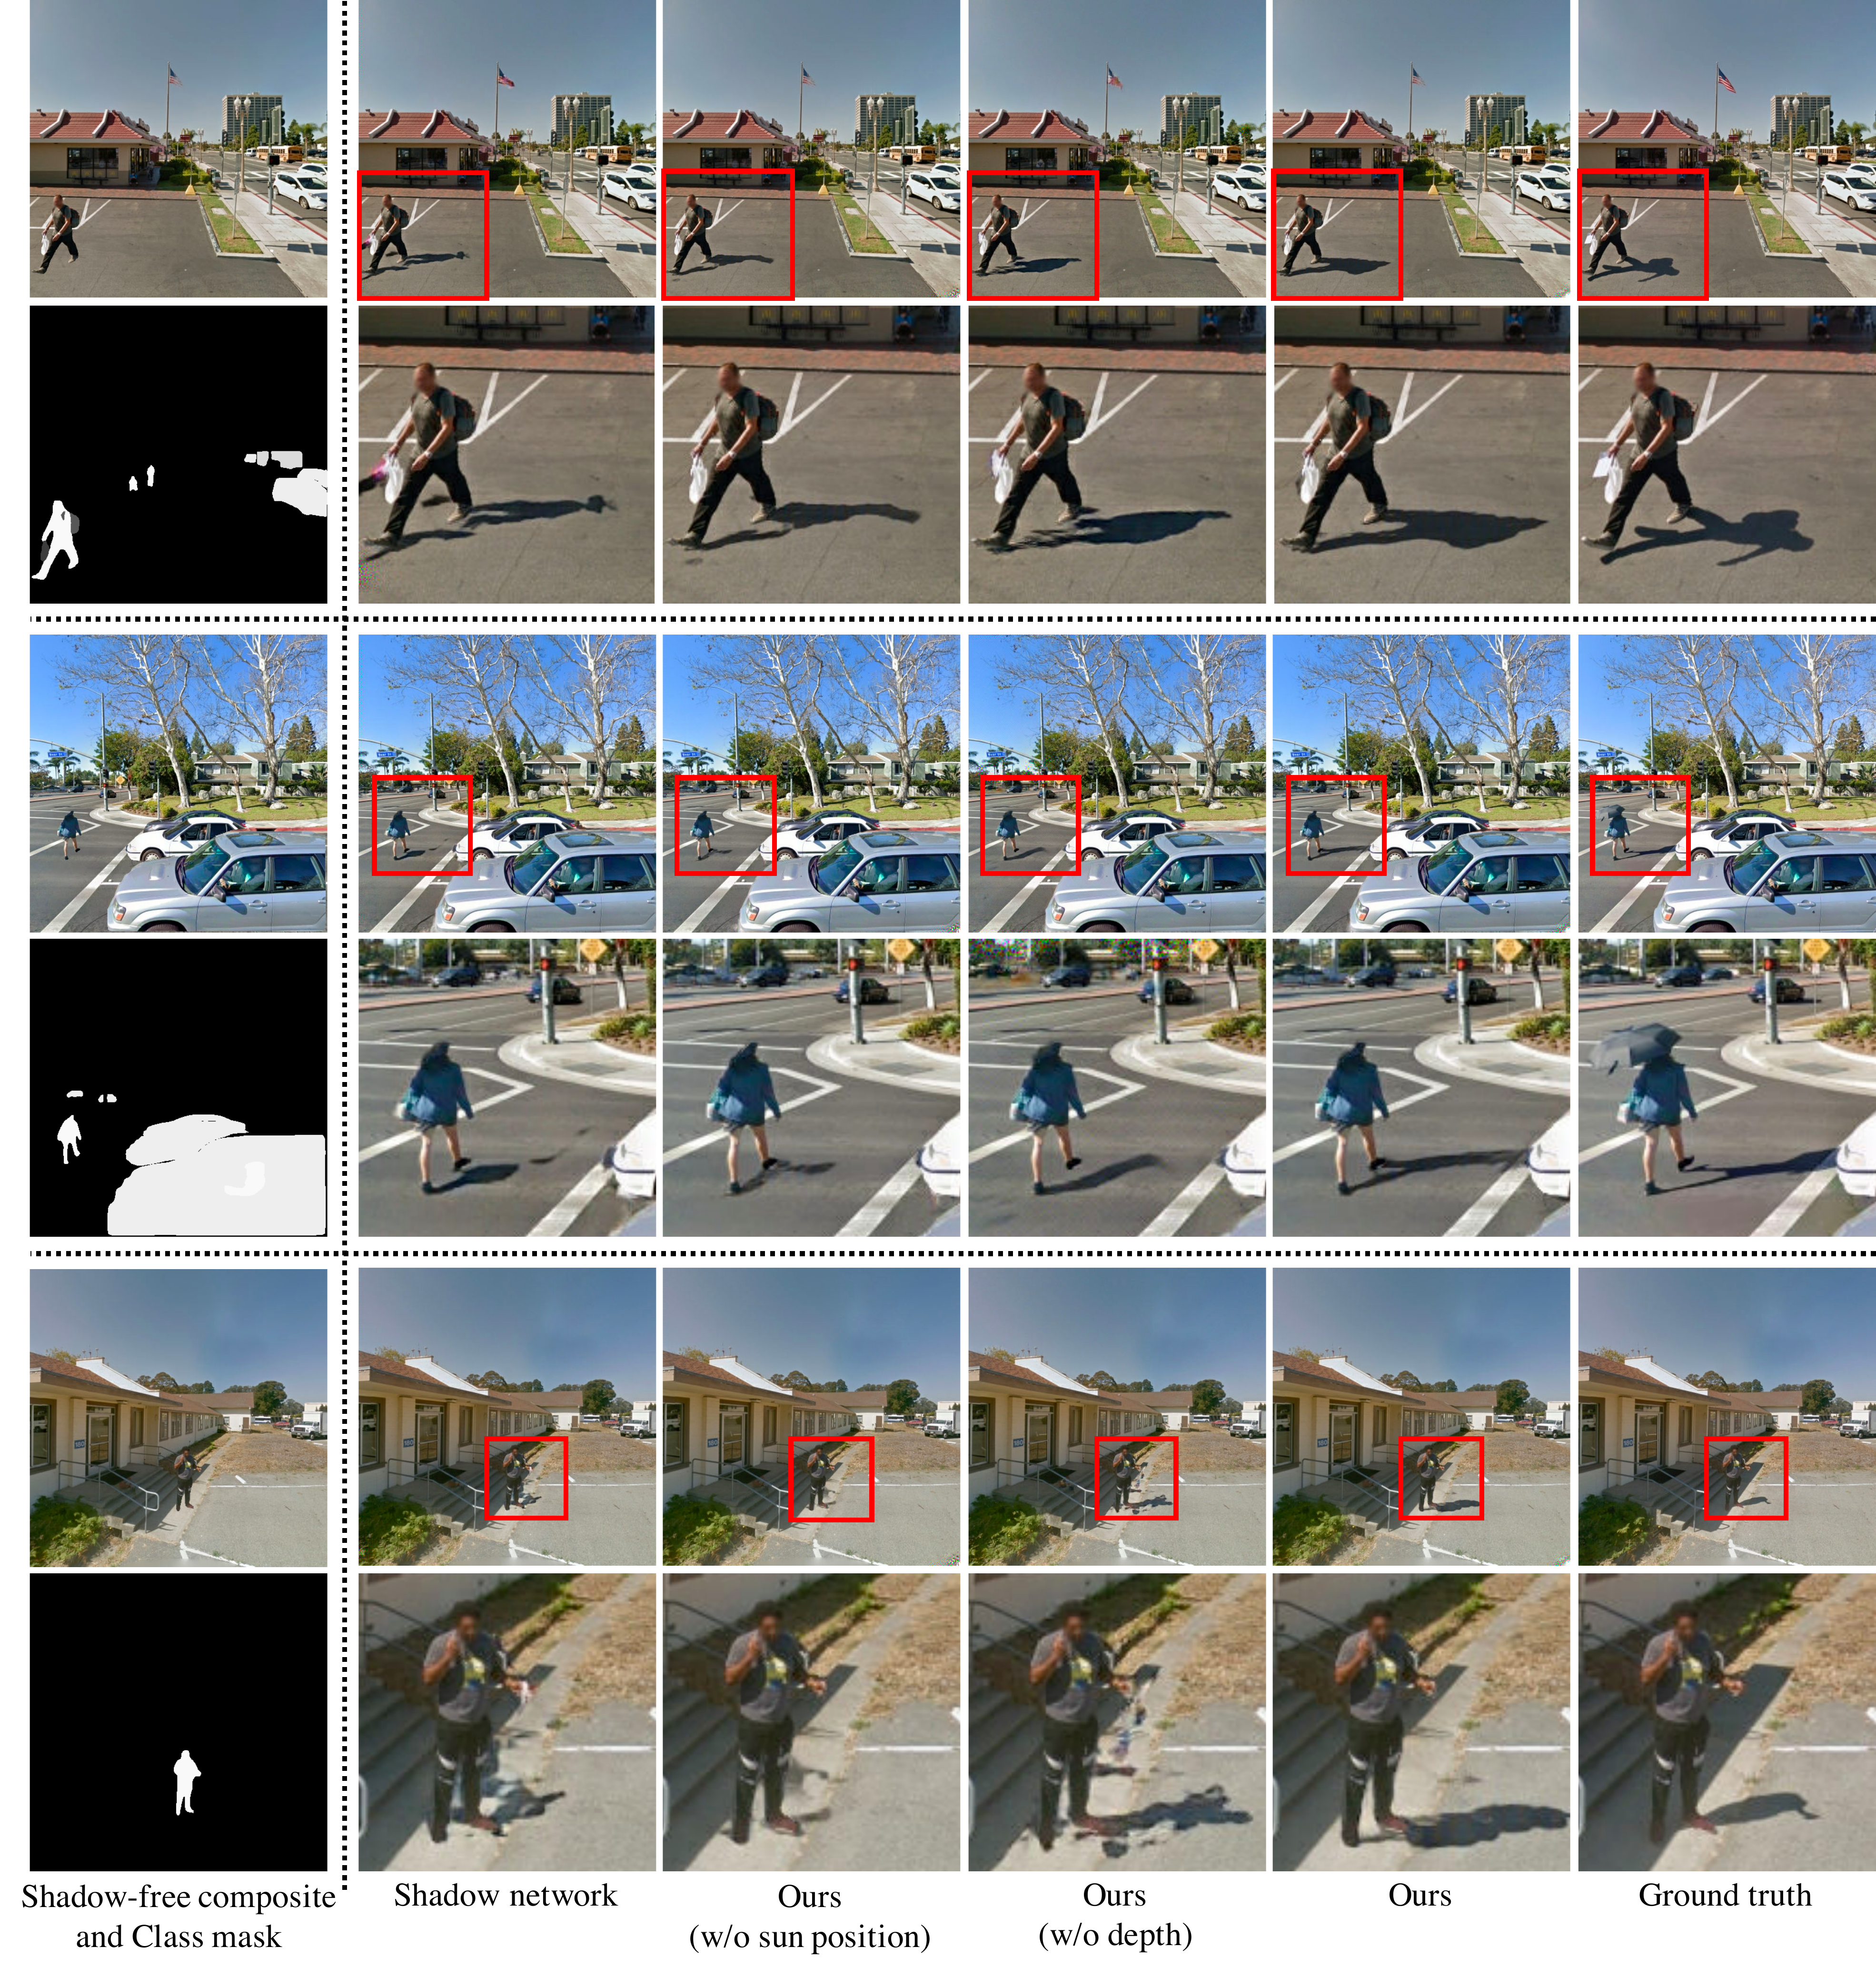}
    \caption{Object insertion results on the test set. Three examples are shown, with red boxes indicating close-up regions. Our method generates the most realistic and detailed shadows. The sun position input helps the network determine the shape of the shadow. The depth maps prevent the network from synthesizing broken shadows.}
    \label{fig:insert_suppl}
\end{figure*}

\begin{figure*}[t]
    \centering
    \includegraphics[width=.9\linewidth]{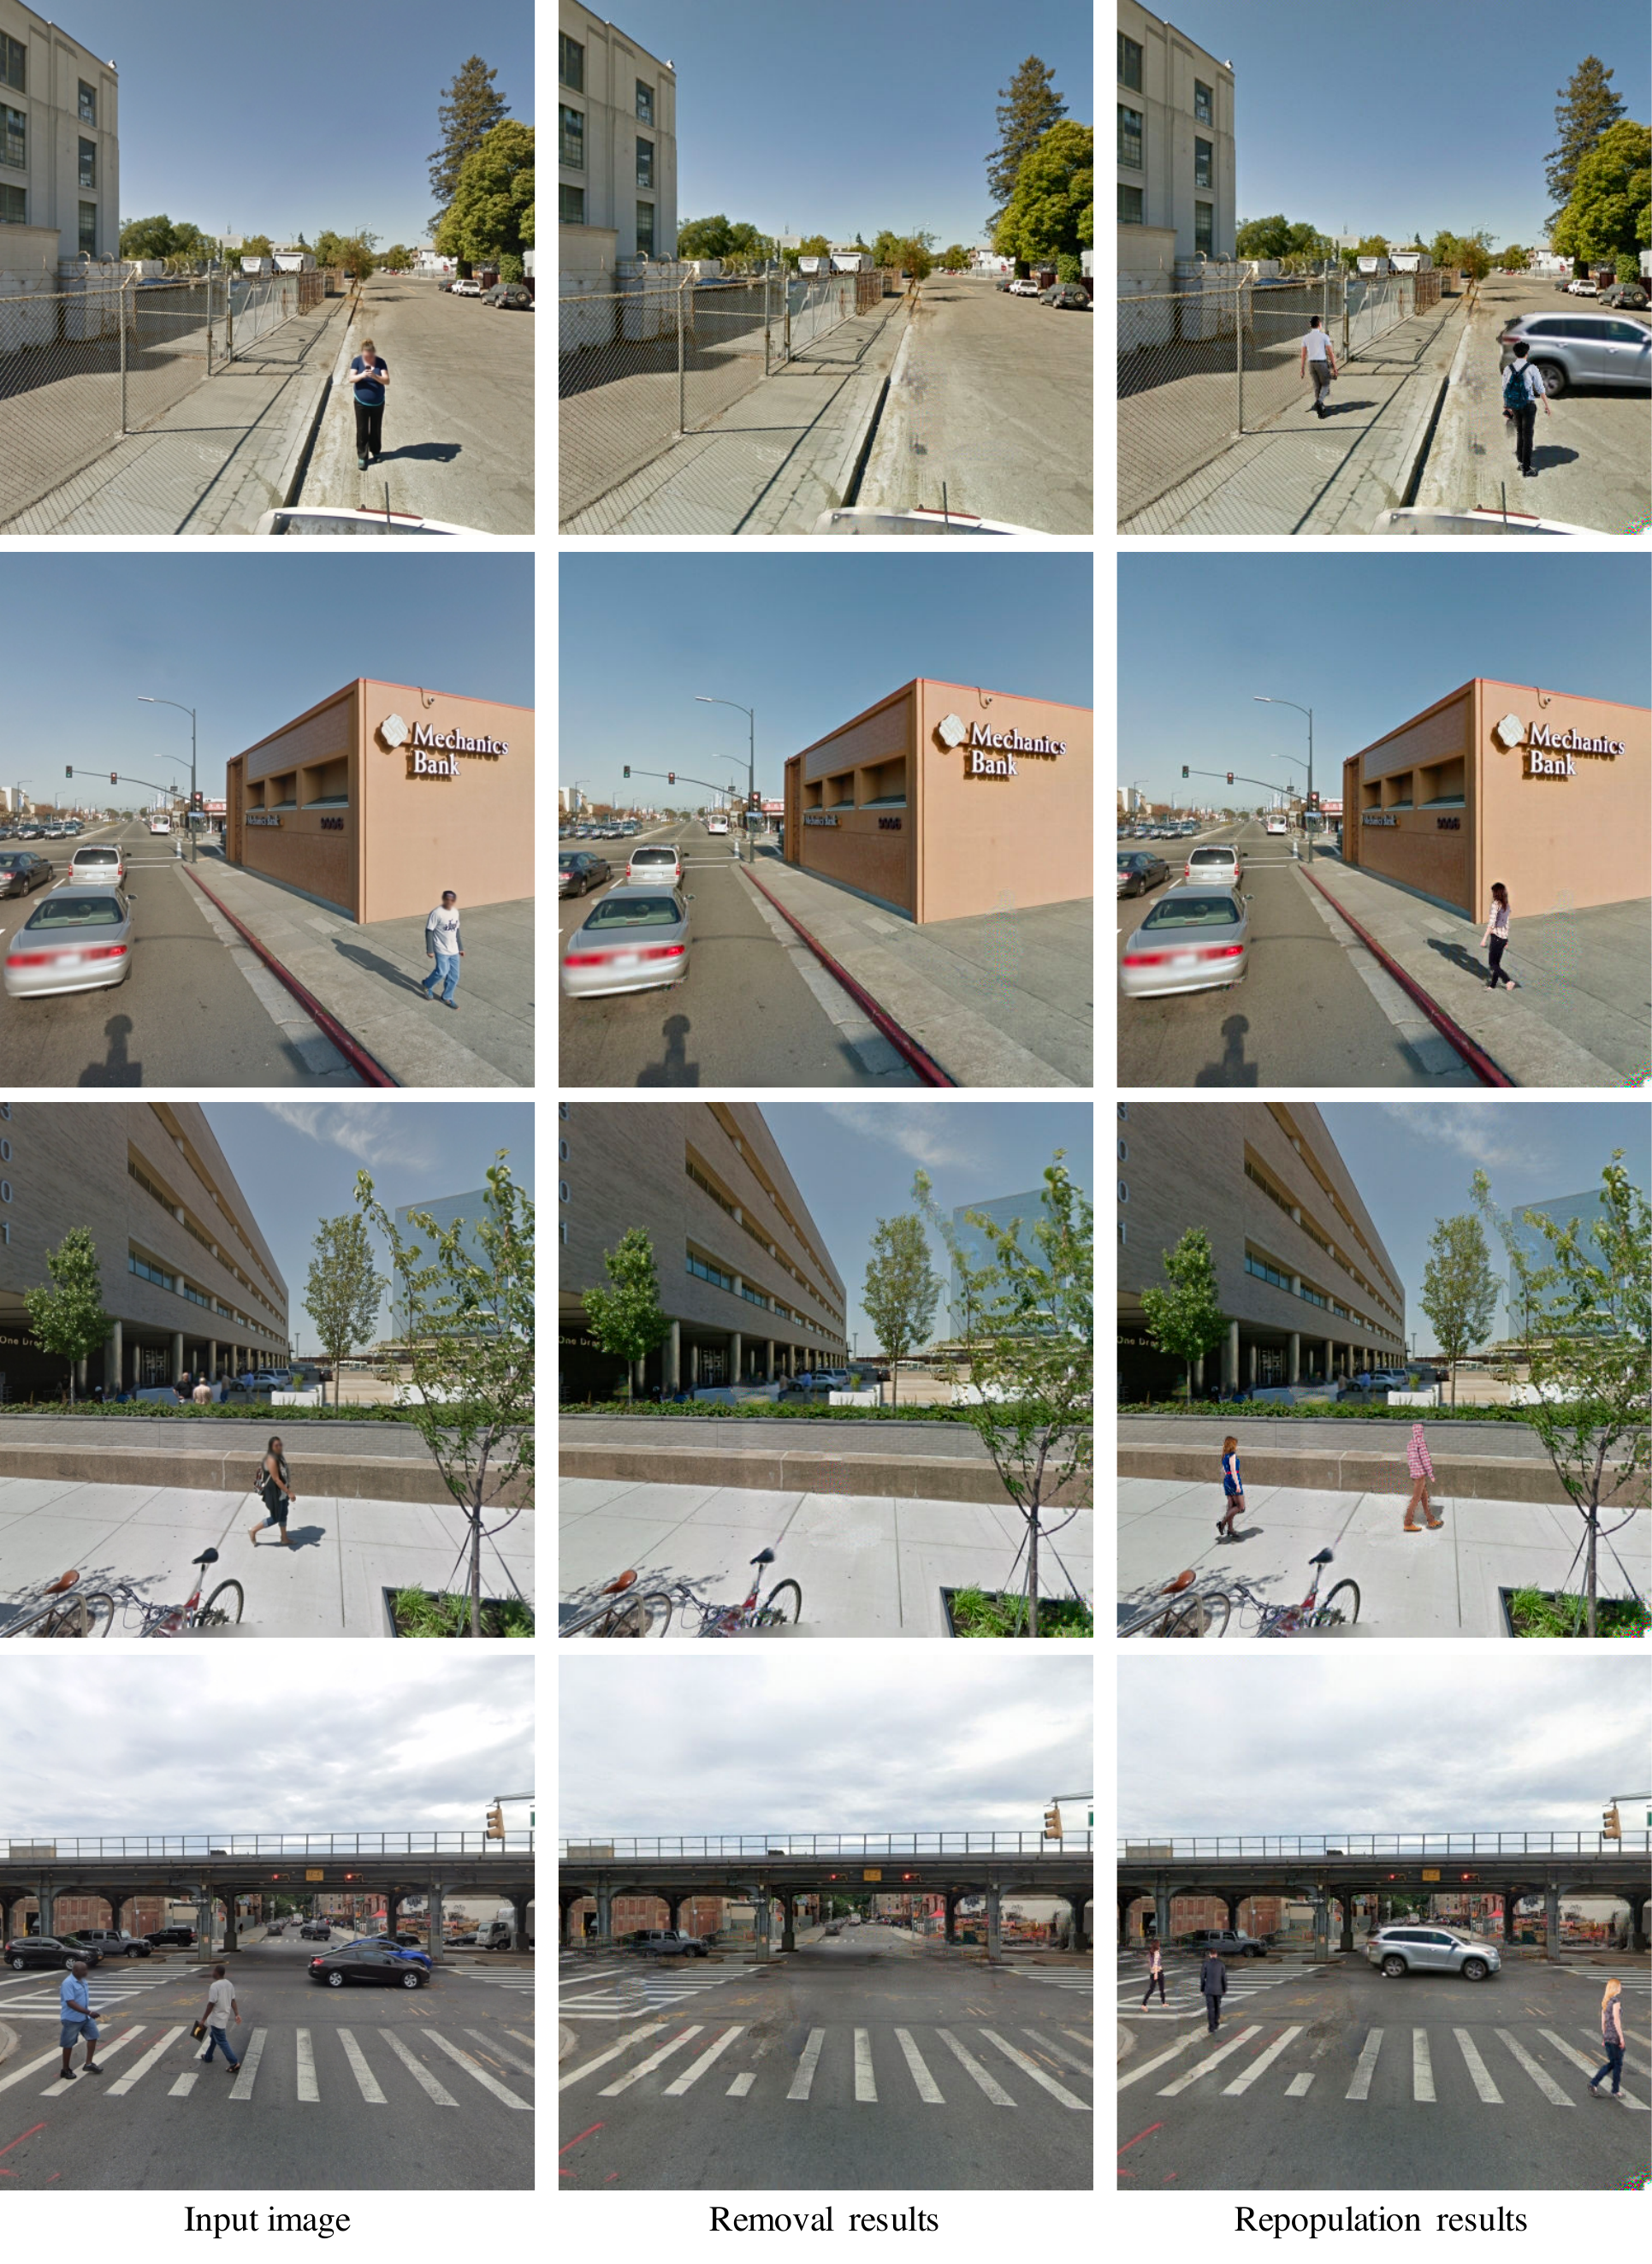}
    \caption{Qualitative results for repopulating street scenes. From left to right: the input image, the background image after removing all people, and repopulation results. Our pipeline selects people matching the scene's lighting, places them randomly on sidewalks and roads, and synthesizes realistic shadows.}
    \label{fig:repop_suppl}
\end{figure*}
